# Supplementary material for: NovelGym: A Flexible Ecosystem for Hybrid Planning and Learning Agents Designed for Open Worlds
Source: arXiv:2401.03546 source file (2024-01-07)
Supplement: Supplementary file 1 [file appendix.tex]

\begin{appendix}

\end{appendix}
